# Supplementary material for: SixthView: A Benchmark for Hidden-View Reconstruction and 3D Assembly Reasoning
Source: arXiv:2611.23891 source file (2026-11-18)
Supplement: Supplementary file 1 [file supplementary.tex]

% Compile this file for the standalone supplement; main.tex builds the paper.
\def\supplementonly{1}
\input{main}
